# Supplementary material for: Heterogeneous integration of silicon nitride and amorphous silicon carbide photonics
Source: arXiv:2507.10312 source file (2025-07-14)
Supplement: Supplementary file 1 [file Supplementary_Material.pdf]

# Heterogeneous integration of silicon nitride and amorphous silicon carbide photonics

Zizheng Li,<sup>1,\*</sup> Bruno Lopez-Rodriguez,<sup>1</sup> Naresh Sharma,<sup>2</sup> Roald van der Kolk,<sup>1</sup> Thomas Scholte,<sup>1</sup> Harmen Smedes,<sup>3</sup> R. Tufan Erdogan,<sup>4</sup> Jin Chang,<sup>3</sup> Hugo Voncken,<sup>1</sup> Jun Gao,<sup>5</sup> Ali W Elshaari,<sup>5</sup> Simon Gröblacher,<sup>3</sup> and Iman Esmail Zadeh<sup>1</sup>

<sup>1</sup>*Department of Imaging Physics (ImPhys), Faculty of Applied Sciences, Delft University of Technology, Delft 2628 CJ, The Netherlands*

<sup>2</sup>*Department of Electronics Engineering, Indian Institute of Technology (Indian School of Mines), Dhanbad, Jharkhand, India*

<sup>3</sup>*Department of Quantum Nanoscience, Faculty of Applied Sciences, Delft University of Technology, Delft 2628 CJ, The Netherlands*

<sup>4</sup>*Department of Precision and Microsystems Engineering, Delft University of Technology, 2628 CD Delft, The Netherlands*

<sup>5</sup>*Department of Applied Physics, KTH Royal Institute of Technology, Albanova University Centre, Stockholm 106 91, Sweden*

(\*Electronic mail: z.l.li-1@tudelft.nl)

## I. Characterization setups

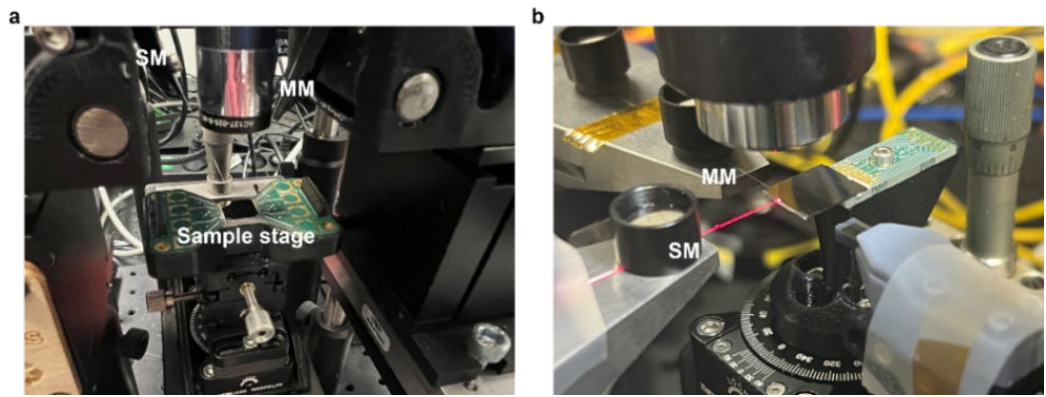

Fig.S1. Optical setups for sample characterization: (a) for grating coupling, (b) for side coupling.

Two kinds of optical setups, for grating-coupling and side-coupling, are used for sample characterization and shown in Fig.S1. As discussed in Fig.3(a) and (b) in the main paper, single-mode fiber (SMF) and multi-mode fiber (MMF) are mounted on the translation stages in both cases, where we use SMF as optical input while MMF for the output. For grating coupling, the input and output fibers are mounted with an 20-degree angle with respect to the sample norm (Fig.S1(a)). For edge coupling, SM fiber and MM fiber are mounted in the sample plane and form a 90-degree angle (Fig.S1(b)). The sample is mounted and pasted on the thermal conductive sample stage that has a proportional integral derivative temperature controller. The sample stage can be installed in both setups.

## II. Fabrication

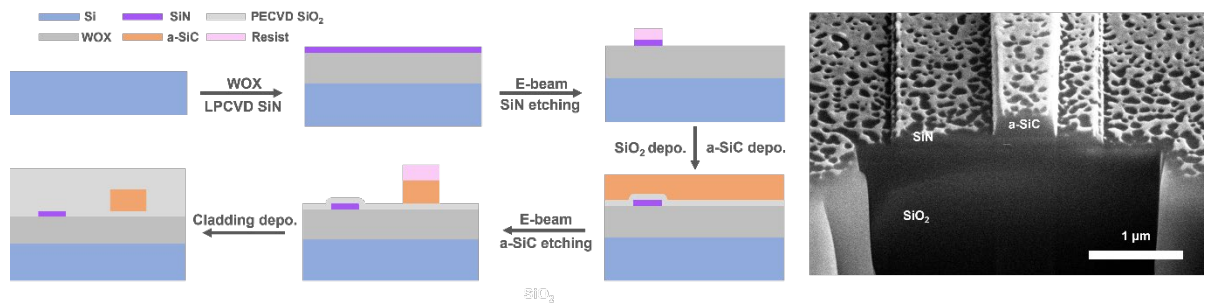

Fig.S2. Heterogeneous a-SiC/SiN PIC fabrication process, and a scanning electron image on a dummy sample showing the a-SiC/SiN cross-section.

The fabrication flow of the a-SiC/SiN heterogeneous PIC platform is illustrated in Fig.S2. The substrate consists of a 4-inch 525 μm thick silicon (Si) wafers with 8 μm wet thermally grown oxide (WOX). A layer of stoichiometric silicon nitride thin film is then deposited on the substrate by LPCVD, aiming for a thickness of 100 nm. The deposition is carried out at 800 °C using dichlorosilane and ammonia (DCS:NH<sub>3</sub> = 1:3) as precursors, under a pressure of 250 mTorr. Owing to the absence and incompatibility of CMP and high temperature annealing (> 1200 °C) in our Kavli Nanolab, these processes are not included in the fabrication flow. The wafer is then cleaved into small samples (in the size of 15 × 15 mm<sup>2</sup>). First, an alignment marker layer is defined (5 nm chromium and 90 nm gold) using standard fabrication with metal lift-off. The resist is stripped in PRS-3000 at 80 °C in a heat bath. Afterwards, to remove the resist residuals we perform a cleaning procedure consisting of oxygen plasma descum, acetone and isopropyl alcohol cleaning in the ultrasonic bath.

To define the SiN waveguides, positive resist ARP 6200-04 is spin-coated on the samples and baked at 160 °C on a hotplate, and subsequently exposed by electron beam lithography (Raith EBPG-5200). After resist development, a post-baking step (130 °C for 1 minute) is performed, for the purpose of reducing the resist sidewall roughness. The patterns on the resist layer are transferred to SiN thin film by reactive-ion etching (RIE, Sentech Etchlab 200), with a gas mixture of fluorine (CHF<sub>3</sub>) and argon (Ar). Succeeding this, we follow the same cleaning procedure mentioned earlier to remove resist residuals. A 40 nm thick SiO<sub>2</sub> layer is deposited on the sample as an isolation layer between SiN and a-SiC via plasma enhanced chemical vapour deposition (PECVD). This layer protects the underlying SiN through the subsequent fabrication steps, maintaining its optical quality.

Thereafter, we deposit a 260 nm a-SiC layer using inductively coupled plasma-enhanced chemical vapour deposition (ICPCVD, Oxford PlasmaPro 100) with mixed precursors of silane (SiH<sub>4</sub>) and methane (CH<sub>4</sub>) at a substrate temperature of 150 °C. Electron beam lithography, resist development, and RIE etching processes are executed again to define the photonic devices on the a-SiC layer. Finally, after resist cleaning, 8 μm PECVD SiO<sub>2</sub> is deposited on top as the optical cladding. The samples are further cleaved using a diamond pen to expose the waveguide cross-sections for side-coupling measurements.

For inspection and imaging purposes, we fabricated an additional sample using the same processes described above, except that exposure and layer-to-layer alignment were performed using a laser-writer instead of electron-beam lithography. We use focused ion beam (FIB) to create an opening at the a-SiC/SiN coupling region, and inspect the layer stack under scanning electron microscopy (SEM), as shown in the right panel of Fig.S2. A clear shift between a-SiC and SiN layers can be seen, which is attributed to the relatively low precision and resolution of the laser-writer. The grains that are visible on the sample surface are the sputtered 20 nm Au film, preventing charging in FIB and SEM processes.

### III. Fabrication tolerance of the a-SiC/SiN interconnection couplers

The most critical parameters for the a-SiC/SiN interconnection couplers are the end-tip widths of the a-SiC and SiN waveguides, which can hugely impact the coupling efficiency. As discussed in the last paragraph of Section. II. A in the main paper, we sweep the end-tip widths in fabrication, and experimentally measured the interconnection coupling efficiencies, as shown in Fig.S3.

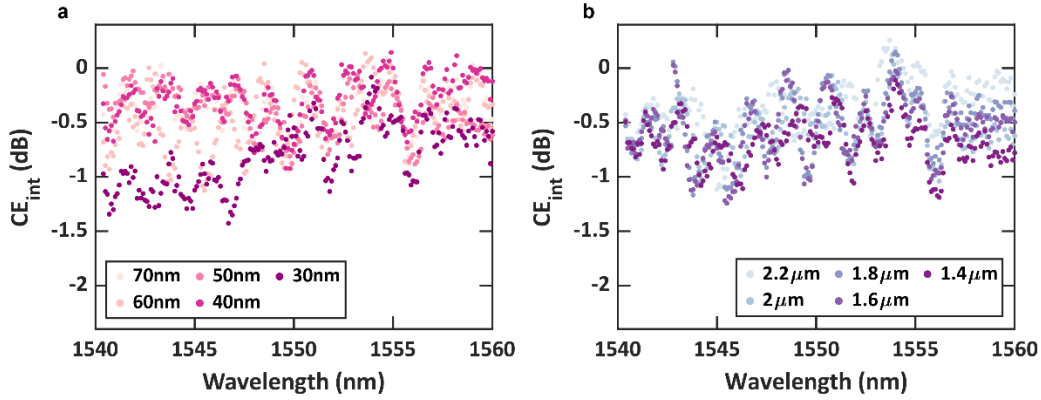

Fig.S3. Fabrication tolerance of the a-SiC/SiN interconnection couplers, when introducing deviations to (a) a-SiC and (b) SiN waveguide end-tip widths.

### IV. Bending losses

The minimal bending radius  $R_{\min}$  is a key performance metric discussed in the main paper, the square of  $R_{\min}$  represents the minimal device area on a photonic chip. To determine the minimal bending radius, we fabricated ring resonators with different bending radii, and measured the resonance spectra. The measured spectra and intrinsic quality factor are shown in Fig.S4. Due to non-optimized ring-bus gaps, the ring resonators are working in varying degrees of the under-coupled regime. Instead of loaded quality factor, we use intrinsic quality factor as the evaluation of bending losses, to eliminate the influence of coupling losses. It is found out that the ring resonators only exhibits pronounced quality factor decrement when bending radius is smaller than  $15 \mu\text{m}$ . Consequently,  $R_{\min} = 15 \mu\text{m}$  is regarded as the minimal bending radius of the a-SiC/SiN PIC.

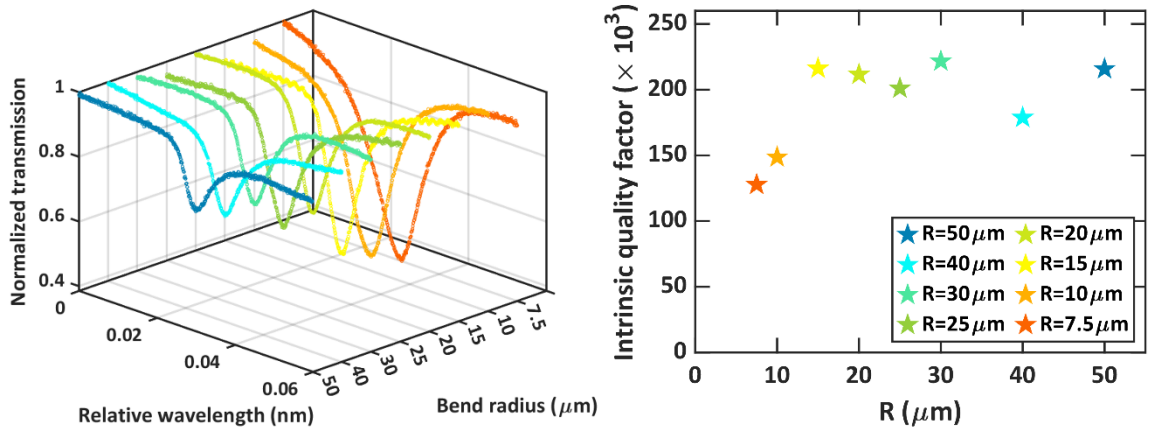

Fig.S4. Spectra measured from ring resonators with different bending radii, and intrinsic quality factors.

## V. Edges couplers on the a-SiC/SiN platform

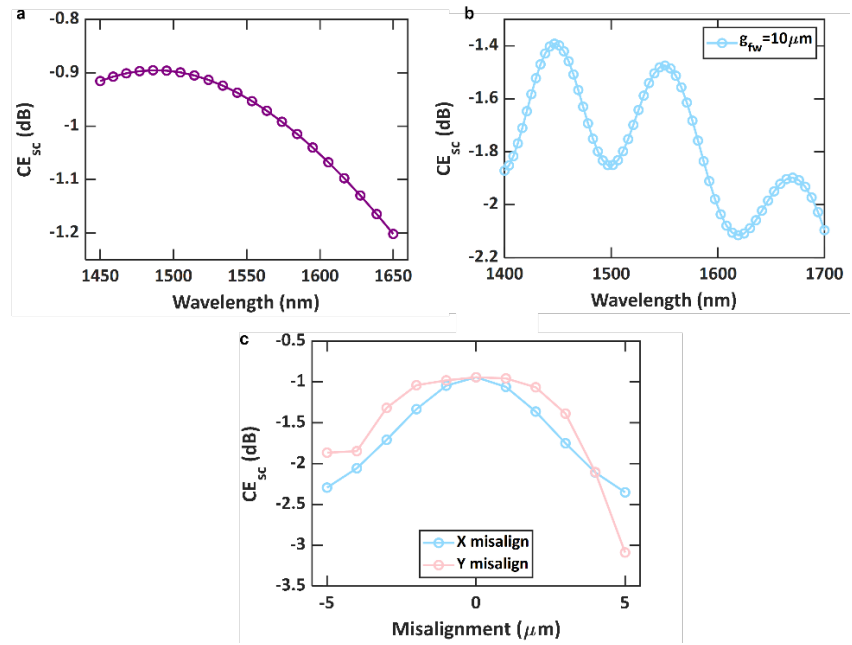

Fig.S5. Simulated results of (a) the coupling efficiency of the inverted taper edge coupler, (b) the edge coupling efficiency when fiber-to-chip air gap = 10  $\mu m$ , (c) the coupling efficiency decrement when the fiber is misaligned.

The simulated coupling efficiency over the wavelength range from 1450 nm to 1650 nm is shown in Fig.S5(a), when the optimal parameters for mode overlapping between fiber and waveguide are applied. Similarly, the definition of edge coupling efficiency corresponds to the  $CE_{sc}$  described in Eq.(4) in the main paper, where standard single mode fiber for 1550 nm is considered in the coupling process. The influences on the edge coupling efficiency due to the fiber-to-chip air gap, and the impact of fiber misalignment in the plane parallel to the sample's cleaved cross-section, are shown in Fig.S5(b) and (c). They are possibly related to the major deviation in the experimental results compared to simulations. Another possible reason, namely the deviations from the sample cleaving process, is presented in Fig.S6. The inherent randomness and uncertainty of sample cleaving determine that the SiN waveguides do not always break at the intended locations. This suggests that further improvements can be achieved through more advanced sample cutting techniques or an additional polishing process.

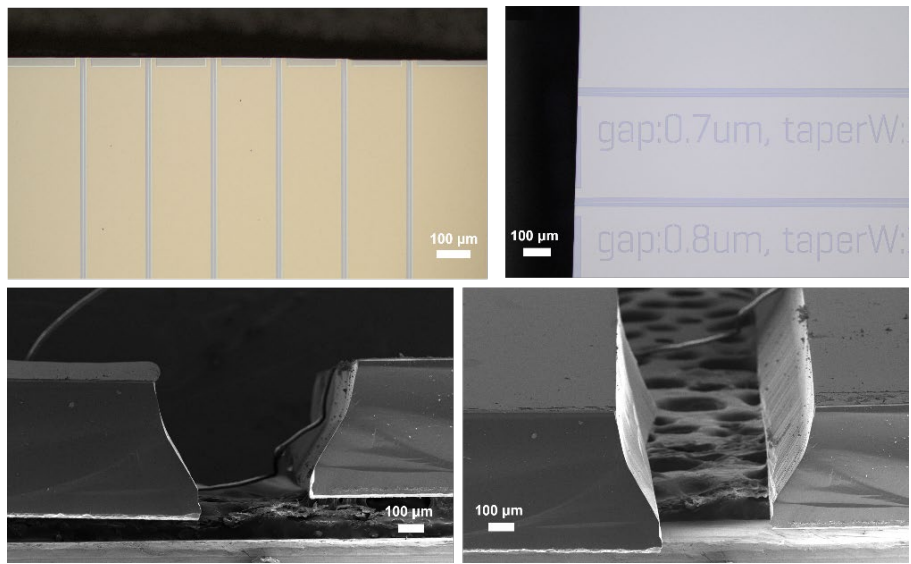

Fig.S6. Optical (top) and scanning electron microscopy (bottom) images of the cleaved sample edges. In the optical microscopy images, the rectangular bars perpendicular to the waveguides are the indicators for the optimal cleaving position.

## VI. Comparison of key performance metrics between different material platforms

Based on the publicly available data and the measured results reported in this work, a comparison of the performance metrics for large-scale tunable photonics between different materials is presented in TABLE I in the main paper. We obtained the waveguide losses of different material platforms from the state-of-the-art literature and the photonic foundries. The device design and heater shape optimization aimed at improving thermos-optic tuning efficiencies are excluded from consideration, when estimating the power consumption for  $\pi$  phase shift, ensuring the comparison focuses solely on the intrinsic properties of each platform.

In TABLE.S1 on the next page, we list the prices of the multi-project wafer (MPW) runs published recently by different photonic foundries. Currency conversions are based on exchange rates as of 5 May 2025. Different foundries have different block definition in MPW, and it largely influences the fabrication price of unit area. In the table, we note the specific block dimensions after the price. We note that the prices cannot be directly compared, since different fabrication techniques are used in different foundries and the performances of fabricated devices are not the identical, and the quantity of the copies that the customer get also varies between foundries. Based on these publicly available multi-project-wafer run prices, equipment and material usage expenses, and operator prices given by photonic foundries, companies and cleanrooms<sup>[1-15]</sup>, we estimate the per minimal-device-area fabrication prices on different PIC platforms (listed in TABLE I). We focus on active photonic integrated circuits that incorporate the waveguides layer and thermos-optic heaters layer, excluding plasma dispersion modulators in Si photonics. The fabrication price for a-SiC/SiN PIC is estimated to be approximately twice of that of the SiN PIC. Given that the two platforms share the same thick oxide layer (10  $\mu\text{m}$   $\text{SiO}_2$ ) on a silicon substrate, and a-SiC layer fabrication is proven to be simple, specifically consisting of chemical vapor deposition, followed by standard lithography and reactive ion etching, the price estimation is believed to be overstated. While the layer-to-layer lithography alignment may cause some extra cost in the a-SiC/SiN fabrication, the additional expense is expected to be lower than the extent of overestimation.

**TABLE.S1 MPW fabrication prices of different platforms from photonic foundries**

|                     | Price per unit area (\$/mm <sup>2</sup> ) for certain block size |                                                                                                     |                                      |                                                                                   |                                                                        |                                                                                |                                          |                                       |
|---------------------|------------------------------------------------------------------|-----------------------------------------------------------------------------------------------------|--------------------------------------|-----------------------------------------------------------------------------------|------------------------------------------------------------------------|--------------------------------------------------------------------------------|------------------------------------------|---------------------------------------|
| <b>PIC platform</b> | Global Foundries                                                 | AIM Photonics                                                                                       | CUMEC                                | imec                                                                              | LioniX                                                                 | CORNERSTONE                                                                    | CNM/<br>VLC<br>Photonics                 | LIGE NTEC                             |
| SOI active          | 9240<br>(5 × 5 mm <sup>2</sup> )                                 | 5363<br>(8 mm <sup>2</sup> )<br><br>3432<br>(25/50/100 mm <sup>2</sup> )                            | 1037<br>(5.15×5.15 mm <sup>2</sup> ) | 1884<br>(5.15×5.15 mm <sup>2</sup> )<br><br>1857<br>(5.15×10.45 mm <sup>2</sup> ) | n.a.                                                                   | 1239<br>(4.9×11.47 mm <sup>2</sup> )<br><br>1551<br>(4.9×5.5 mm <sup>2</sup> ) | n.a.                                     | n.a.                                  |
| SOI passive         | n.a.                                                             | 1373<br>(8 mm <sup>2</sup> )<br><br>1030<br>(50 mm <sup>2</sup> )<br><br>686 (100 mm <sup>2</sup> ) | 249<br>(5.15×5.15 mm <sup>2</sup> )  | 548<br>(5.15×5.15 mm <sup>2</sup> )<br><br>479<br>(5.15×10.45 mm <sup>2</sup> )   | n.a.                                                                   | 229<br>(4.9×11.47 mm <sup>2</sup> )<br><br>332<br>(4.9×5.5 mm <sup>2</sup> )   | n.a.                                     | n.a.                                  |
| SOI with heater     | n.a.                                                             | 5363<br>(8 mm <sup>2</sup> )<br><br>3432<br>(25/50/100 mm <sup>2</sup> )                            | 385<br>(5.15×10.38 mm <sup>2</sup> ) | 548<br>(5.15×5.15 mm <sup>2</sup> )<br><br>479<br>(5.15×10.45 mm <sup>2</sup> )   | n.a.                                                                   | 362<br>(4.9×11.47 mm <sup>2</sup> )<br><br>557<br>(4.9×5.5 mm <sup>2</sup> )   | n.a.                                     | n.a.                                  |
| SiN with heater     | n.a.                                                             | 5363<br>(8 mm <sup>2</sup> )<br><br>3432<br>(25/50/100 mm <sup>2</sup> )                            | Unknown                              | Unknown                                                                           | 226<br>(10×10 mm <sup>2</sup> )<br><br>170<br>(10×20 mm <sup>2</sup> ) | 115<br>(11.47×15.45 mm <sup>2</sup> )                                          | 398.22<br>(5×5 or 5×10 mm <sup>2</sup> ) | 507.9<br>7<br>(5×10 mm <sup>2</sup> ) |
| SiN passive         | n.a.                                                             | 686<br>(50 mm <sup>2</sup> )                                                                        | Unknown                              | Unknown                                                                           | 226<br>(10×10 mm <sup>2</sup> )<br><br>170<br>(10×20 mm <sup>2</sup> ) | 62<br>(11.47×15.45 mm <sup>2</sup> )                                           | 398.22<br>(5×5 / 5×10 mm <sup>2</sup> )  | 507.9<br>7<br>(5×10 mm <sup>2</sup> ) |

## References

1. EURORACTICE-IC. Schedules & Prices 2024. EURORACTICE-IC. <https://europactice-ic.com/schedules-prices-2024> (accessed 05 May 2025).
2. Cornerstone Photonics Foundry. Cornerstone Photonics Fabrication Services. Cornerstone Photonics. <https://www.cornerstone.sotonfab.co.uk/> (accessed 05 May 2025).
3. AIM Photonics. AIM Photonics Multi-Project Wafer Services. AIM Photonics. <https://www.aimphotonics.com/> (accessed 05 May 2025).
4. JePPIX Foundry Network. JePPIX European Photonic Foundries. JePPIX. <https://www.jeppix.eu/foundries/> (accessed 05 May 2025).
5. MIT Nano Users. FabNano Photonic Integration Facility. MIT. <https://nanousers.mit.edu/fabnano/> (accessed 05 May 2025).
6. Rogue Valley Microdevices. Photonic Integrated Circuit Fabrication. Rogue Valley Microdevices. <https://roguevalleymicrodevices.com> (accessed 05 May 2025).
7. Stanford Nanofabrication Facility. SNF Photonics Fabrication. Stanford University. <https://snf.stanford.edu/> (accessed 05 May 2025).
8. JD Photodata. Photonic Device Fabrication Services. JD-Photodata. <https://www.jd-photodata.co.uk/> (accessed 05 May 2025).
9. AnySilicon. Die-per-Wafer Formula & Free Calculators. AnySilicon. <https://anysilicon.com/die-per-wafer-formula-free-calculators/> (accessed 05 May 2025).
10. Imec Photonic Integration Platform. Imec. <https://www.imec-int.com> (accessed 05 May 2025).
11. LioniX International. Photonics Foundry Services. LioniX International. <https://www.lionix-international.com/photonics/> (accessed 05 May 2025).
12. Ligentec. Integrated Photonics Foundry. Ligentec. <https://www.ligentec.com/> (accessed 05 May 2025).
13. MIT Nano Users. FabNano Photonic Integration Facility. MIT. <https://nanousers.mit.edu/fabnano/> (accessed 05 May 2025).
14. IMB-CNM Integrated Micro and Nanofabrication Clean Room. Silicon Nitride Photonic Integration Platform. IMB-CNM. <https://www.imb-cnm.csic.es/en/micro-and-nanofabrication-clean-room/silicon-nitride-photonic-integration-platform> (accessed 05 May 2025).
15. CUMEC. Micro-Nano Fabrication. CUMEC. [http://www.cumec.cn/en/menu\\_4.html](http://www.cumec.cn/en/menu_4.html) (accessed 05 May 2025).
